# Supplementary material for: Scalable Approximate Inference and Some Applications
Source: arXiv:2003.03515 source file (2020-03-07)
Supplement: Supplementary file 1 [file appendix.tex]

\begin{appendices}
\section*{Appendicies}

\section{Detail of Network Architecture}
We use the same AlexNet as \citet{zhu2018binary}, which is illustrated in the following.
{\small 
\begin{table}[h]
    \centering
    \begin{tabular}{|c|c|c|} \hline
    Layer & Type & Parameters \\\hline
     1    & Conv & Depth: 96, K: $11\times 11$, S: 4, P:0 \\
     2  &  Relu &  - \\
     3 & MaxPool & K: $3\times 3$, S: 2 \\
     4 & BatchNorm & -  \\
     5 & Conv & Depth: 256, K: $5\times 5$, S: 1, P:1 \\
    6  &  Relu &  - \\
      7 & MaxPool & K: $3\times 3$, S: 2 \\
     8 & BatchNorm & -  \\
     9 & Conv & Depth: 384, K: $3\times 3$, S: 1, P:1 \\
     10  &  Relu &  - \\
     11 & Conv & Depth: 384, K: $3\times 3$, S: 1, P:1 \\
    12  &  Relu &  - \\
    13 & Conv & Depth: 256, K: $3\times 3$, S: 1, P:1 \\
    14  &  Relu &  - \\
    15 & MaxPool & K: $3\times 3$, S: 2 \\
    16  &Dropout & $p=0.5$\\
    17  & FC & Width=4096\\
     18  &  Relu &  - \\
    19  &Dropout & $p=0.5$\\
    20  & FC & Width=4096\\
    21  &  Relu &  - \\
    22 & FC & Width=10\\\hline
    \end{tabular}
    \caption{Architecture of AlexNet. "K" denotes kernel size; "S" denotes stride; "P" denotes padding.}
    \label{tab:alexnet}
\end{table}
}

\end{appendices}
